# Supplementary material for: Communication Optimization for Decentralized Learning atop Bandwidth-limited Edge Networks
Source: arXiv:2504.12210 source file (2025-04-21)
Supplement: Supplementary file 1 [file appendix.tex]

\addcontentsline{toc}{section}{Appendices}

\subsection{Supporting Proofs}\label{appendix:Proofs}

\begin{proof}[Proof of Lemma~\ref{lem:equal bandwidth allocation}]
The rate of each multicast flow $h\in H$ is determined by the minimum rate of the unicast flows constituting it. Consider the bottleneck underlay link $\ue^* := \argmin_{\ue\in \uE} C_{\ue}/t_{\ue}$. Since there are $t_{\ue^*}$ unicast flows sharing a total bandwidth of $C_{\ue^*}$ at $\ue^*$, the slowest of these flows cannot have a rate higher than $C_{\ue^*}/t_{\ue^*}$. Thus, the multicast flow containing this slowest unicast flow cannot have a rate higher than $C_{\ue^*}/t_{\ue^*}$, which means that the completion time for all the multicast flows is no smaller than \eqref{eq:tau - special case, per-link}. 

Meanwhile, if the bandwidth of every link is shared equally among the activated unicast flows traversing it, then each unicast flow will receive a bandwidth allocation of no less than $C_{\ue^*}/t_{\ue^*}$ at every hop, and thus can achieve a rate of at least $C_{\ue^*}/t_{\ue^*}$. Hence, each multicast flow $h\in H$ can achieve a rate of at least $C_{\ue^*}/t_{\ue^*}$, yielding a completion time of no more than \eqref{eq:tau - special case, per-link}. 
\end{proof}

\begin{proof}[Proof of Lemma~\ref{lem:equal bandwidth allocation - category}]
According to Lemma~\ref{lem:equal bandwidth allocation}, it suffices to prove that $\min_{F\in \mathcal{F}} C_F/t_F = \min_{\ue\in \uE} C_{\ue}/t_{\ue}$. To this end, we first note that by Definition~\ref{def: category}, all the underlay links in the same category must be traversed by the same set of overlay links and thus the same set of activated unicast flows, i.e., $t_{\ue} = t_F$ $\forall \ue\in \Gamma_F$. By the definition of the category capacity $C_F$, we have 
\begin{align}
\min_{\ue\in \Gamma_F} {C_{\ue}\over t_{\ue}} = \min_{\ue\in \Gamma_F} {C_{\ue}\over t_F} = {C_F\over t_F}.
\end{align}
Thus, we have
\begin{align}
\min_{\ue\in \uE} {C_{\ue}\over t_{\ue}} = \min_{F\in \mathcal{F}} \min_{\ue\in \Gamma_F} {C_{\ue}\over t_{\ue}} = \min_{F\in \mathcal{F}} {C_F\over t_F}. 
\end{align}
\end{proof}

\begin{proof}[Proof of Corollary~\ref{cor:optimal link weights}]
As $K(p,1)$ decreases with $p$, its minimum is achieved at the maximum value of $p$ that satisfies \eqref{eq:condition on p} for $t=1$ and any value of $\bm{X}$, i.e., 
\begin{align}
    p := \min_{\bm{X}\neq \bm{0}} \left(1-{\E[\|\bm{X}(\bm{W}-\bm{J})\|_F^2]\over \|\bm{X}(\bm{I}-\bm{J})\|_F^2}\right).\label{eq:p-maximization objective}
\end{align}
By \cite[Lemma~3.1]{Xusheng24ICASSP}, $p$ defined in \eqref{eq:p-maximization objective} satisfies $p = 1-\tilde{\rho}$ for $\tilde{\rho} := \|\E[\bm{W}^\top\bm{W}]-\bm{J}\|$. By Jensen's inequality and the convexity of $\|\cdot\|$, $\tilde{\rho} \leq \E[\|\bm{W}^\top \bm{W} - \bm{J}\|]$. 
For every realization of $\bm{W}$ that is symmetric with rows/columns summing to one, %in the form of $\bm{I}-\bm{B}\diag(\bm{\alpha})\bm{B}^\top$, 
we have $\bm{W}^\top\bm{W}-\bm{J}=(\bm{W}-\bm{J})^2$. Based on the eigendecomposition $\bm{W}-\bm{J} = \bm{Q}\diag(\lambda_1,\ldots,\lambda_m)\bm{Q}^\top$, we have\looseness=-1 
\begin{align}
\|\bm{W}^\top\bm{W}-\bm{J}\| &= \|\bm{Q}\diag(\lambda_1^2,\ldots,\lambda_m^2)\bm{Q}^\top \| \nonumber\\
& = \max_{i=1,\ldots,m} \lambda_i^2 = \|\bm{W}-\bm{J}\|^2, 
\end{align}
where we have used the fact that $\|\bm{W}-\bm{J}\| = \max_{i=1,\ldots,m}|\lambda_i|$. 
%\yudi{Does $ \| \cdot \|$ denote the spectral norm?}\ting{yes, see Section~\ref{subsec:Notations}.} 
Thus, $K(p,1)$ for $p$ defined in \eqref{eq:p-maximization objective} is upper-bounded by $K(1- \E[\|\bm{W}-\bm{J}\|^2], 1)$, which is a sufficient number of iterations for D-PSGD to achieve $\epsilon_0$-convergence by Theorem~\ref{thm:new convergence bound}. 

The matrix inequality \eqref{wo cost:matrix} implies that $\rho\geq |\lambda_i|$ for all $i=1,\ldots,m$, and thus the optimal value of \eqref{eq:min rho wo cost} must satisfy $\rho = \max_{i=1,\ldots,m}|\lambda_i| = \|\bm{W}-\bm{J}\|$. Hence, the optimal value $\rho^*$ of \eqref{eq:min rho wo cost} is the minimum value of $\| \bm{W}-\bm{J}\|$ for any realization of $\bm{W}$ that only activates the links in $E_a$. Therefore, $1-\E[\|\bm{W}-\bm{J}\|^2]\leq 1- \mathop{\rho^*}^2$ and \eqref{eq:relaxed bound on K} $\geq K(1- \mathop{\rho^*}^2,1)$, with ``$=$'' achieved at $\bm{W}^* = \bm{I}-\bm{B}\diag(\bm{\alpha}^*)\bm{B}^\top$. 
\end{proof}

\begin{proof}[Proof of Lemma~\ref{lem:equivalence to bilevel}]
Let $(\beta^*, E_a^*)$ be the optimal solution to the RHS of \eqref{eq:equivalance to bilevel}, and $E_a^o$ be the optimal solution to the LHS of \eqref{eq:equivalance to bilevel}. Let $\beta^o:= \overline{\tau}(E_a^o)$. Then
\begin{align}
&\min_{\overline{\tau}(E_a)\leq \beta^o}\overline{K}(E_a) \leq \overline{K}(E_a^o) \\
\Rightarrow& \beta^o \cdot \left(\min_{\overline{\tau}(E_a)\leq \beta^o}\overline{K}(E_a) \right) \leq \overline{\tau}(E_a^o)\cdot \overline{K}(E_a^o) \\
\Rightarrow& \min_{\beta\geq 0} \beta \cdot \left(\min_{\overline{\tau}(E_a)\leq \beta} \overline{K}(E_a) \right)\leq \overline{\tau}(E_a^o)\cdot \overline{K}(E_a^o). \label{eq:equivalence proof - 1}
\end{align}
Meanwhile, $\beta^*$ must equal $\overline{\tau}(E_a^*)$, as otherwise we can reduce $\beta^*$ to further reduce the value of $\beta \cdot \left(\min_{\overline{\tau}(E_a)\leq \beta} \overline{K}(E_a) \right)$, contradicting with the assumption that $(\beta^*, E_a^*)$ is optimal. Therefore, by the definition of $E_a^o$,
\begin{align}
\min_{\beta\geq 0} \beta \cdot \left(\min_{\overline{\tau}(E_a)\leq \beta} \overline{K}(E_a) \right) &= \overline{\tau}(E_a^*) \cdot \overline{K}(E_a^*) \nonumber\\
&\geq \overline{\tau}(E_a^o)\cdot \overline{K}(E_a^o), \label{eq:equivalence proof - 2}
\end{align}
which together with \eqref{eq:equivalence proof - 1} proves \eqref{eq:equivalance to bilevel}.

Moreover, \eqref{eq:equivalance to bilevel} implies that ``$=$'' must hold for \eqref{eq:equivalence proof - 2}, i.e., $E_a^*$ is also optimal for the LHS of \eqref{eq:equivalance to bilevel}. 
\end{proof}

\begin{proof}[Proof of Lemma~\ref{lem:reduction to algebraic connectivity}]
It suffices to prove that under condition \eqref{eq:requirement on alpha^0}, \eqref{eq:bound rho - 2} is achieved at $1-\lambda_2(\bm{L}(E_a)),\: \forall E_a\subseteq \widetilde{E}$, i.e., $\lambda_2(\bm{L}(E_a)) + \lambda_m(\bm{L}(E_a))\leq 2$. 

By definition, $\lambda_m(\bm{L}(E_a)) = \max\{\bm{v}^\top \bm{L}(E_a)\bm{v}:\: \|\bm{v}\|=1\}$. Also by definition, $\bm{L}(E_a) = \bm{D}(E_a) - \bm{A}(E_a)$, where $\bm{D}(E_a)$ and $\bm{A}(E_a)$ are the degree matrix and the adjacency matrix for a weighted graph with link weights $\bm{\alpha}^{(0)}(E_a)$. We have
\begin{align}
\bm{v}^\top \bm{D}(E_a) \bm{v} &= \sum_{i=1}^m v_i^2 \sum_{j: (i,j)\in E_a}\alpha^{(0)}_{ij} \nonumber\\
&\leq \max_{i\in V}\sum_{j: (i,j)\in \widetilde{E}}\alpha^{(0)}_{ij}, \label{eq:proof - algebraic - 1}
\end{align}
because $\sum_{i=1}^m v_i^2 = 1$ and $\sum_{j: (i,j)\in E_a}\alpha^{(0)}_{ij} \leq \sum_{j: (i,j)\in \widetilde{E}}\alpha^{(0)}_{ij}$. 
Moreover, we also have
\begin{align}
-\bm{v}^\top \bm{A}(E_a) \bm{v} &\leq \sum_{i,j=1}^m |(A(E_a))_{ij}|\cdot |v_i|\cdot |v_j| \nonumber \\
&\leq (\max_{(i,j)\in \widetilde{E}}|\alpha^{(0)}_{ij}|) \sqrt{\sum_{i,j=1}^m v_i^2} \sqrt{\sum_{i,j=1}^m v_j^2} \label{eq:proof - algebraic - 2} \\
&= m \cdot \max_{(i,j)\in \widetilde{E}}|\alpha^{(0)}_{ij}|, \label{eq:proof - algebraic - 3}
\end{align}
where \eqref{eq:proof - algebraic - 2} is because of $|(A(E_a))_{ij}|\leq \max_{(i,j)\in \widetilde{E}}|\alpha^{(0)}_{ij}|$ and the Cauchy-Schwarz inequality, and \eqref{eq:proof - algebraic - 3} is because $\sum_{i=1}^m v_i^2 = \sum_{j=1}^m v_j^2 = 1$. 
Combining \eqref{eq:requirement on alpha^0}, \eqref{eq:proof - algebraic - 1}, and \eqref{eq:proof - algebraic - 3} implies that $\bm{v}^\top \bm{L}(E_a)\bm{v} \leq 1$ for any unit-norm vector $\bm{v}$. Thus, $\lambda_2(\bm{L}(E_a))\leq \lambda_m(\bm{L}(E_a))\leq 1$, completing the proof. 
\end{proof}

\begin{proof}[Proof of Theorem~\ref{thm:overall solution}]
Under the assumption of $\widehat{\mathcal{F}}\supseteq \mathcal{F}$ and $\widehat{C}_F \leq C_F$ ($\forall F\in \mathcal{F}$), every real (per-category) capacity constraint is ensured by a capacity constraint we formulate based on the inferred parameters $\widehat{\mathcal{F}}$ and $(\widehat{C}_F)_{F\in \widehat{\mathcal{F}}}$, and thus any communication schedule that is feasible under the inferred constraints remains feasible under the actual constraints. This implies that the proposed design  predicted to complete each iteration in time $\overline{\tau}(E_a^*)$ can actually complete each iteration within this time. 
Moreover, by Corollary~\ref{cor:optimal link weights}, D-PSGD under the designed mixing matrix achieves $\epsilon_0$-convergence within $K(E_a^*)$ iterations, which is further bounded by $\overline{K}(E_a^*)$ according to \eqref{eq:K_bound}. Thus, D-PSGD under the proposed design can achieve $\epsilon_0$-convergence within time $\overline{\tau}(E_a^*) \cdot \overline{K}(E_a^*)$.  
\end{proof}
